# Supplementary material for: Connection between $GW$ and Extended Coupled Cluster
Source: arXiv:2602.10887 ancillary file (2026-06-04)
Supplement: Supplementary file 1 [file si.pdf]

# Supplementary Material for “Connection between $GW$ and Extended Coupled Cluster”

Johannes Tölle,<sup>1, a)</sup> Marios-Petros Kitsaras,<sup>2, b)</sup> Andreas Irmmler,<sup>3, c)</sup> Andreas Grüneis,<sup>3, d)</sup> and Pierre-François Loos<sup>2, e)</sup>

<sup>1)</sup>Department of Chemistry, University of Hamburg, 22761 Hamburg, Germany; The Hamburg Centre for Ultrafast Imaging (CUI), Hamburg 22761, Germany

<sup>2)</sup>Laboratoire de Chimie et Physique Quantiques (UMR 5626), Université de Toulouse, CNRS, Toulouse, France

<sup>3)</sup>Institute for Theoretical Physics, TU Wien, Wiedner Hauptstraße 8-10/136, Vienna, Austria

This **Supplementary Material** provides the derivations and working equations supporting the connection between the  $GW$  approximation and the extended coupled-cluster (ECC) framework introduced in the main text. We present key amplitude identities, the full spin-adapted EOM  $\sigma$ -vector equations (including the  $G_0W_0$ -TDA subset and ECC-based vertex corrections), and the perturbative ECC formulation of the linearized one-body  $GW$  density matrix.

## I. AMPLITUDE RELATIONS

To demonstrate the following relation

$$\mathbf{1} + \mathbf{z} + \mathbf{t} \cdot \mathbf{z} = (\mathbf{1} - \mathbf{t})^{-1} \quad (1)$$

we start by rewriting the left-hand side as

$$\mathbf{1} + \mathbf{z} + \mathbf{t} \cdot \mathbf{z} = \mathbf{1} + \mathbf{t} \cdot (\mathbf{1} - \mathbf{t} \cdot \mathbf{t})^{-1} + \mathbf{t} \cdot \mathbf{t} \cdot (\mathbf{1} - \mathbf{t} \cdot \mathbf{t})^{-1} \quad (2)$$

where we made use of<sup>1</sup>

$$\begin{aligned} \mathbf{z} &= \mathbf{Y} \cdot (\mathbf{X} - \mathbf{t} \cdot \mathbf{Y})^{-1} \\ &= \mathbf{t} \cdot (\mathbf{1} - \mathbf{t} \cdot \mathbf{t})^{-1} \end{aligned} \quad (3)$$

Realizing that the right-hand side of Eq. (2) can be recast into a von-Neumann series

$$\begin{aligned} \mathbf{1} + \mathbf{t} \cdot (\mathbf{1} - \mathbf{t} \cdot \mathbf{t})^{-1} + \mathbf{t} \cdot \mathbf{t} \cdot (\mathbf{1} - \mathbf{t} \cdot \mathbf{t})^{-1} \\ = \mathbf{1} + \sum_{k=0}^{\infty} \mathbf{t}^{2k+1} + \sum_{k=0}^{\infty} \mathbf{t}^{2k+2} \\ = \sum_{k=0}^{\infty} \mathbf{t}^k = (\mathbf{1} - \mathbf{t})^{-1} \end{aligned} \quad (4)$$

establishes the relationship in Eq. (1).

## II. $\sigma$ -VECTOR EQUATIONS

The spin-adapted  $\sigma$ -vector equations for the  $m$ th excitation vector in the EOM eigenvalue problem defined in Eq. 46 for the doubly similarity-transformed electron-boson Hamiltonian, are presented in Sec. II A. The additional vertex corrections to the  $G_0W_0$  approximation within the EOM-ECC framework are presented in Sec. II B.

The Einstein summation convention is implied over all repeated indices throughout. Electron repulsion integrals are defined in chemists' notation as  $V_{pqrs} = (pq|rs)$ . Furthermore, composite electron-hole fermionic indices, denoted as  $\nu, \mu, \dots$  in the manuscript, are resolved into occupied ( $i, j, k, l, m, n, \dots$ ) and virtual ( $a, b, c, d, e, f, \dots$ ) fermionic indices. Consequently, the amplitude tensors  $\mathbf{t}$  and  $\mathbf{z}$  are defined as  $t_{\nu\mu} = t_{ijab}$  and  $z_{\nu\mu} = z_{ijab}$ , the excitation vectors as  $r_{iv}^{(m)} = r_{ijb}^{(m)}$  and  $r_{va}^{(m)} = r_{jba}^{(m)}$ .

### A. EOM-ECC working equations

A subset of the full EOM-ECC  $\sigma$ -vector equations corresponds to the  $G_0W_0$   $\sigma$ -vector equations within the Tamm-Dancoff approximation (TDA). The equations were first presented in Ref. 2, and are provided here for completeness. The  $\sigma$ -vector equations for  $G_0W_0$  within the TDA read

$$\sigma_i^{(m)} = f_{ij}r_j^{(m)} + f_{ia}r_a^{(m)} + 2V_{iabj}r_{jba}^{(m)} + 2V_{kijb}r_{kjb}^{(m)} \quad (5a)$$

$$\begin{aligned} \sigma_{ijb}^{(m)} &= V_{icbj}r_c^{(m)} + V_{jbki}r_k^{(m)} \\ &\quad - f_{bc}r_{ijc}^{(m)} + f_{ki}r_{kjb}^{(m)} + f_{ij}r_{ilb}^{(m)} - 2V_{lcbj}r_{ilc}^{(m)} \end{aligned} \quad (5b)$$

$$\sigma_a^{(m)} = f_{ab}r_b^{(m)} + f_{ai}r_i^{(m)} + 2V_{jbca}r_{jbc}^{(m)} + 2V_{iajb}r_{ijb}^{(m)} \quad (5c)$$

$$\begin{aligned} \sigma_{jba}^{(m)} &= V_{jbca}r_c^{(m)} + V_{jbai}r_i^{(m)} \\ &\quad + f_{ca}r_{jbc}^{(m)} + f_{cb}r_{jca}^{(m)} + f_{ij}r_{iba}^{(m)} + 2V_{jbck}r_{kca}^{(m)} \end{aligned} \quad (5d)$$

Next, the direct-ring ECC  $\sigma$ -vector equations containing the contraction with  $\mathbf{t}$  and  $\mathbf{z}$  are presented. The direct contractions with the amplitudes  $\mathbf{t}$  read

$$\sigma_i^{(m)}[t] = 4V_{lcai}t_{lkcd}r_{kda}^{(m)} \quad (6a)$$

$$\begin{aligned} \sigma_{ijb}^{(m)}[t] &= 2V_{kcai}t_{kjb}r_a^{(m)} + 2V_{laki}t_{ljab}r_a^{(m)} \\ &\quad - 4V_{lcka}t_{kjab}r_{ilc}^{(m)} \end{aligned} \quad (6b)$$

$$\sigma_a^{(m)}[t] = 4V_{icba}t_{ikcd}r_{kdb}^{(m)} \quad (6c)$$

$$\sigma_{jba}^{(m)}[t] = 4V_{jbic}t_{ikcd}r_{kda}^{(m)} \quad (6d)$$

<sup>a)</sup>Electronic mail: johannes.toelle@uni-hamburg.de

<sup>b)</sup>Electronic mail: kitsaras@irsamc.ups-tlse.fr

<sup>c)</sup>Electronic mail: andreas.irmmler@tuwien.ac.at

<sup>d)</sup>Electronic mail: andreas.gruneis@tuwien.ac.at

<sup>e)</sup>Electronic mail: loos@irsamc.ups-tlse.fr

while the direct contractions with the amplitudes  $\mathbf{z}$  are

$$\sigma_i^{(m)}[z] = 4V_{raki}z_{lrca}r_{klc}^{(m)} \quad (7a)$$

$$\sigma_a^{(m)}[z] = 4V_{kabi}z_{licb}r_{klc}^{(m)} \quad (7b)$$

$$\sigma_{jba}^{(m)}[z] = 2V_{scda}z_{jsbc}r_d^{(m)} + 2V_{kacs}z_{jsbc}r_k^{(m)} \quad (7c)$$

Lastly, the direct-ring contractions containing both  $\mathbf{t}$  and  $\mathbf{z}$  amplitudes are given by

$$\sigma_i^{(m)}[t, z] = 8V_{kcmi}z_{jled}t_{klcd}r_{mje}^{(m)} \quad (8a)$$

$$\sigma_a^{(m)}[t, z] = 8V_{makc}z_{jled}t_{klcd}r_{mje}^{(m)} \quad (8b)$$

$$\sigma_{jba}^{(m)}[t, z] = 4V_{kcea}z_{jlbd}t_{klcd}r_e^{(m)} + 4V_{iakc}z_{jlbd}t_{klcd}r_i^{(m)} \quad (8c)$$

## B. Vertex corrections within EOM-ECC

As explained in the manuscript (Sec. VIII), the direct-ring  $\sigma$ -vector equations are modified to include exchange contributions in three distinct ways:

(i) Exchange corrections in the two-electron integrals ( $\Gamma_V^x$ ):

$$\sigma_i^{(m)} = -V_{ibaj}r_{jba}^{(m)} - V_{kbji}r_{kjb}^{(m)} \quad (9a)$$

$$\sigma_{ijb}^{(m)} = V_{ljbc}r_{ilc}^{(m)} \quad (9b)$$

$$\sigma_a^{(m)} = -V_{jcba}r_{jbc}^{(m)} - V_{ibja}r_{ijb}^{(m)} \quad (9c)$$

$$\sigma_{jba}^{(m)} = -V_{jckb}r_{kca}^{(m)} \quad (9d)$$

$$\sigma_i^{(m)}[t] = -2V_{liac}t_{lkcd}r_{kda}^{(m)} \quad (9e)$$

$$\sigma_{ijb}^{(m)}[t] = -V_{kipc}t_{kjb}r_p^{(m)} - V_{kali}t_{ljab}r_j^{(m)} \quad (9f)$$

$$+ 2V_{lalc}t_{kjab}r_{ilc}^{(m)} \quad (9g)$$

$$\sigma_a^{(m)}[t] = -2V_{iabc}t_{ikcd}r_{kdb}^{(m)} \quad (9h)$$

$$\sigma_{jba}^{(m)}[t] = -2V_{jcib}t_{ikcd}r_{kda}^{(m)} \quad (9i)$$

$$\sigma_i^{(m)}[z] = -2V_{ibkj}z_{ljcb}r_{klc}^{(m)} \quad (9j)$$

$$\sigma_a^{(m)}[z] = -2V_{kjba}z_{ljcb}r_{klc}^{(m)} \quad (9k)$$

$$\sigma_{jba}^{(m)}[z] = -V_{icda}z_{jlbd}r_c^{(m)} - V_{kida}z_{jlbd}r_k^{(m)} \quad (9l)$$

$$\sigma_i^{(m)}[z, t] = -4V_{mcki}z_{jled}t_{klcd}r_{mje}^{(m)} \quad (9m)$$

$$\sigma_a^{(m)}[z, t] = -4V_{mcka}z_{jled}t_{klcd}r_{mje}^{(m)} \quad (9n)$$

$$\sigma_{jba}^{(m)}[z, t] = -2V_{kace}z_{jlbd}t_{klcd}r_e^{(m)} - 2V_{icka}z_{jlbd}t_{klcd}r_i^{(m)} \quad (9n)$$

(ii) Exchange corrections in the amplitudes ( $\Gamma_A^x$ ):

$$\sigma_i^{(m)}[t] = -2V_{ldai}t_{lkcd}r_{kca}^{(m)} \quad (10a)$$

$$\sigma_{ijb}^{(m)}[t] = -V_{kdai}t_{kjb}r_a^{(m)} - V_{lcki}t_{ljbc}r_k^{(m)} \quad (10b)$$

$$+ 2V_{lckd}t_{kjb}r_{ilc}^{(m)} \quad (10c)$$

$$\sigma_a^{(m)}[t] = -2V_{idba}t_{ikcd}r_{kcb}^{(m)} \quad (10d)$$

$$\sigma_{jba}^{(m)}[t] = -2V_{jbid}t_{ikcd}r_{kca}^{(m)} \quad (10e)$$

$$\sigma_i^{(m)}[z] = -2V_{jbki}z_{ljcb}r_{klc}^{(m)} \quad (10f)$$

$$\sigma_a^{(m)}[z] = -2V_{kabj}z_{ljcb}r_{klc}^{(m)} \quad (10g)$$

$$\sigma_{jba}^{(m)}[z] = -V_{lcda}z_{jlcb}r_d^{(m)} - V_{kacj}z_{jlcb}r_k^{(m)} \quad (10g)$$

(iii) Exchange corrections in both ( $\Gamma_{CR}^x$ ):

$$\sigma_i^{(m)}[t] = V_{liad}t_{lkcd}r_{kca}^{(m)} \quad (11a)$$

$$\sigma_{ijb}^{(m)}[t] = V_{kjad}t_{kibd}r_a^{(m)} - V_{kclj}t_{libc}r_k^{(m)} \quad (11b)$$

$$- V_{ldkc}t_{kjb}r_{ilc}^{(m)} \quad (11c)$$

$$\sigma_a^{(m)}[t] = V_{iabd}t_{ikcd}r_{kcb}^{(m)} \quad (11d)$$

$$\sigma_{jba}^{(m)}[t] = V_{jdib}t_{ikcd}r_{kca}^{(m)} \quad (11e)$$

$$\sigma_i^{(m)}[z] = -2V_{jbki}z_{ljcb}r_{klc}^{(m)} \quad (11f)$$

$$\sigma_a^{(m)}[z] = -2V_{kabj}z_{ljcb}r_{klc}^{(m)} \quad (11g)$$

$$\sigma_{jba}^{(m)}[z] = -V_{lcda}z_{jlcb}r_d^{(m)} - V_{kacj}z_{jlcb}r_k^{(m)} \quad (11h)$$

$$\sigma_i^{(m)}[t, z] = -4V_{mcki}z_{jled}t_{klcd}r_{mje}^{(m)} \quad (11i)$$

$$\sigma_a^{(m)}[t, z] = -4V_{mcka}z_{jled}t_{klcd}r_{mje}^{(m)} \quad (11j)$$

$$\sigma_{jba}^{(m)}[t, z] = -2V_{kace}z_{jlbd}t_{klcd}r_e^{(m)} - 2V_{icka}z_{jlbd}t_{klcd}r_i^{(m)} \quad (11j)$$

## III. LINEARIZED DENSITY MATRIX

The amplitude equations (Sec. IX) for the linearized one-body  $GW$  density matrix within the ECC perturbation theory framework are

$$0 = V_{ia,v}(\delta_{v,\mu} + 2t_{v,\mu}) + A_{\mu,v}t_{ia,v}^{(1)} + f_{ab}t_{ib,\mu}^{(1)} - f_{ji}t_{ja,\mu}^{(1)} + 2B_{\mu,v}t_{v,\lambda}t_{ia,\lambda}^{(1)} \quad (12)$$

for  $t_{ia,\mu}^{(1)}$ , and

$$0 = f_{ia} + f_{ab}t_{ib}^{(2)} - f_{ji}t_{ja}^{(2)} - 2V_{ij,v}(\delta_{v,\mu} + 2z_{v,\mu} + 4t_{v,\lambda}z_{\lambda,\mu})t_{ja,\mu}^{(1)} + 2V_{ab,v}(\delta_{v,\mu} + 2z_{v,\mu} + 4t_{v,\lambda}z_{\lambda,\mu})t_{ib,\mu}^{(1)} \quad (13)$$

for  $t_{ia}^{(2)}$ . The elements  $A_{\mu,\mu}$  are defined as

$$A_{\mu,\mu} = A_{ia,jb} = \delta_{ij}f_{ab} - \delta_{ab}f_{ij} + B_{ia,jb}, \quad (14)$$

with  $B_{\mu,v} = B_{ia,jb} = 2V_{ia,jb}$ . The amplitude equations for  $z_{ia,\mu}^{(1)}$  read

$$0 = V_{ia,v}(\delta_{v,\mu} + 2z_{v,\mu} + 4t_{v,\lambda}z_{\lambda,\mu}) + A_{\mu,v}z_{ia,v}^{(1)} + f_{ab}z_{ib,\mu}^{(1)} - f_{ji}z_{ja,\mu}^{(1)} + 2B_{\mu,v}t_{v,\lambda}z_{ia,\lambda}^{(1)} \quad (15)$$

and  $z_{ia}^{(2)}$  is obtained from

$$0 = f_{ia} + f_{ab}z_{ib}^{(2)} - f_{ji}z_{ja}^{(2)} - 2V_{ij,v}(\delta_{v,\mu} + 2t_{v,\mu})z_{ja,\mu}^{(1)} + 2V_{ab,v}(\delta_{v,\mu} + 2t_{v,\mu})z_{ib,\mu}^{(1)} \quad (16)$$

Based on the above equations, the linearized one-body  $GW$  density matrix within ECC is computed as  $\gamma^{GW}$

$$\gamma^{GW} = \gamma^\dagger + \gamma, \quad (17)$$

with

$$\gamma_{ij} = 2\delta_{ij} - 2t_{ja,\mu}^{(1)} z_{ia,\mu}^{(1)} \quad (18a)$$

$$\gamma_{ab} = 2t_{ia,\mu}^{(1)} z_{ib,\mu}^{(1)} \quad (18b)$$

$$\gamma_{ia} = t_{ia}^{(2)} \quad (18c)$$

$$\gamma_{ai} = z_{ia}^{(2)} \quad (18d)$$

We have ensured that the resulting natural occupation numbers from  $\gamma^{GW}$  within the ECC framework are identical to those obtained from the linearized  $GW$  density matrix presented in Refs. 3–5 [see Eqs. (57a)–(57c)].

## REFERENCES

<sup>1</sup>M.-P. Kitsaras, J. Tölle, and P.-F. Loos, “Analytic g0w0 gradients based on a double-similarity transformation equation-of-motion coupled-cluster

treatment,” *J. Chem. Phys.* **164**, 044122 (2026).

<sup>2</sup>S. J. Bintrim and T. C. Berkelbach, “Full-frequency gw without frequency,” *J. Chem. Phys.* **154**, 041101 (2021).

<sup>3</sup>F. Bruneval, “Improved density matrices for accurate molecular ionization potentials,” *Phys. Rev. B* **99**, 041118 (2019).

<sup>4</sup>F. Bruneval, “Assessment of the linearized gw density matrix for molecules,” *J. Chem. Theory Comput.* **15**, 4069–4078 (2019).

<sup>5</sup>F. Bruneval, M. Rodriguez-Mayorga, P. Rinke, and M. Dvorak, “Improved one-shot total energies from the linearized gw density matrix,” *J. Chem. Theory Comput.* **17**, 2126–2136 (2021).
